# Supplementary material for: Extending the WILDS Benchmark for Unsupervised Adaptation
Source: arXiv:2112.05090 source file (2022-04-24)
Supplement: Supplementary file 1 [file app_splits.tex]

\section{Experiments on other unlabeled splits}\label{sec:app_splits}

TODO: Move this section up

\begin{table}[th]
\caption{}
\label{tab:splits_results}
\centering
\begin{tabular}{lrr}
\toprule
                       & \multicolumn{2}{c}{\Amazon}                          \\
                       & \multicolumn{2}{c}{(10th percentile acc)}            \\
                       \cmidrule{2-3}
                       & \multicolumn{2}{c}{Masked LM}                        \\
                       & In-distribution            & Out-of-distribution     \\
Unlabeled target       & 71.9 (0.4)                 & 53.9 (0.7)              \\
Unlabeled extra        & 72.0 (0.3)                 & \textbf{54.7} (0.0)     \\
\midrule
                       & \multicolumn{2}{c}{\FMoW}                            \\
                       & \multicolumn{2}{c}{(Worst-region acc)}               \\
                       \cmidrule{2-3}
                       & \multicolumn{2}{c}{NoisyStudent}                     \\
                       & In-distribution            & Out-of-distribution     \\
Unlabeled target       & 61.3 (0.4)                 & \textbf{37.8} (0.6)     \\
Unlabeled validation   & 58.0 (0.7)                 & \textbf{38.2} (0.1)     \\
Unlabeled train        & 55.3 (0.5)                 & 35.7 (1.3)              \\
\midrule
                       & \multicolumn{2}{c}{\Camelyon}                        \\
                       & \multicolumn{2}{c}{(Average acc)}                    \\
                       \cmidrule{2-3}
                       & \multicolumn{2}{c}{NoisyStudent}                     \\
                       & In-distribution            & Out-of-distribution     \\
Unlabeled target       & 93.2 (0.5)                 & \textbf{86.7} (1.7)     \\
Unlabeled validation   & 92.1 (0.9)                 & \textbf{87.6} (4.0)     \\
Unlabeled train        & 92.1 (1.7)                 & 77.8 (3.9)              \\
                       \cmidrule{2-3}
                       & \multicolumn{2}{c}{SwAV}                             \\
                       & In-distribution            & Out-of-distribution     \\
Unlabeled target       & 92.3 (0.4)                 & \textbf{91.4} (2.0)     \\
Unlabeled validation   & 93.2 (0.4)                 & \textbf{91.9} (2.2)     \\
Unlabeled train        & 93.4 (0.3)                 & \textbf{91.1} (1.8)     \\
\bottomrule
\end{tabular}
\end{table}
